# Supplementary material for: Integration of Quantum Accelerators with High Performance Computing -- A Review of Quantum Programming Tools
Source: arXiv:2309.06167 source file (2023-09-18)
Supplement: Supplementary file 1 [file appendix.tex]

\section{Basic Quantum Gates}\label{app:sec:quantum_gates}
 
Graphically, a single qubit $\ket{\psi}$ can be represented as a point on the so-called \emph{Bloch sphere}: 
$\ket{\psi} = \cos(\theta) \ket{0} + e^{i\phi} \sin(\theta) \ket{1}$, illustrated in \autoref{fig:BS}.
\begin{figure}[H]
    \centering
    \includegraphics[scale=0.7]{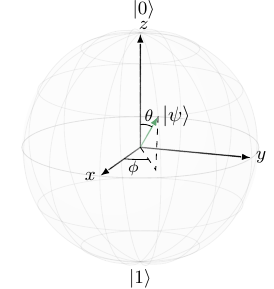}
    \caption{The Bloch sphere.}
    \Description{A sphere with radius 1 that is at the origin of a three-dimensional coordinate system. The x-axis goes to the direction of the reader, the y-axis to the right, and the z-axis to the top. The north and south pole (corresponding to positive and negative Z) are labeled with $\ket{0}$ and $\ket{1}$, respectively. 
    A vector labeled $\ket{\psi}$ points to a point on the surface of the sphere. The vector is defined by the angles $\phi$ (starting at the positive x-axis, going counterclockwise in the x-y-plane) and $\theta$ (starting from the positive z-axis, going clockwise to the ``end-vector'' of angle $\psi$.)}
    \label{fig:BS}
\end{figure}%
The sphere is defined in a typical three-dimensional coordinate system with a x-,y-, and z-axis. The point $\ket{\psi}$ is defined by $\phi$ (angle on the x-y-plane starting from the positive x-axis and going counter-clockwise) and $\theta$ (angle starting from the positive z-axis and going clockwise to the ``end-vector'' of angle $\ket{\psi}$).

The qubit states \(\ket{0} \text{ and } \ket{1}\) correspond to the vectors on the Z-axis, as marked in the sphere.

The behavior of single-qubit gates can be explained in terms of the Bloch sphere. A brief explanation of the gates discussed in this work is given in the following table:
\begin{center}
    \scriptsize
    \begin{tabular}{ccl}
    \toprule
        Gate & Matrix & Explanation \\
        \midrule
        X & $\begin{pmatrix}0 & 1 \\ 1 & 0\end{pmatrix}$ & $180^{\circ}$-rotation around the X-axis of the Bloch sphere \\
        Y & $\begin{pmatrix}0 & i \\ -i & 0\end{pmatrix}$ & $180^{\circ}$-rotation around the Y-axis of the Bloch sphere \\
        Z & $\begin{pmatrix}1 & 0 \\ 0 & -1\end{pmatrix}$ & $180^{\circ}$-rotation around the Z-axis of the Bloch sphere \\
        H & $\frac{1}{\sqrt{2}}\begin{pmatrix}1 & 1 \\ 1 & -1\end{pmatrix}$ & \parbox[]{0.75\textwidth}{$180^{\circ}$-rotation around the X+Z-axis of the Bloch sphere; leads to a uniformly distributed superposition when applied to one of the computational basis states%
        }  \\
        \midrule
        CNOT & $\begin{pmatrix} 1 & 0 & 0 & 0 \\ 0 & 1 & 0 & 0 \\ 0 & 0 & 0 & 1 \\ 0 & 0 & 1 & 0 \end{pmatrix}$ & Application of an X-gate on the second qubit (target qubit) conditioned by the first qubit (control qubit) \\
        SWAP & $\begin{pmatrix} 1 & 0 & 0 & 0 \\ 0 & 0 & 1 & 0 \\ 0 & 1 & 0 & 0 \\ 0 & 0 & 0 & 1 \end{pmatrix}$ & Exchange of the states of two given qubits \\
        \bottomrule
    \end{tabular}
\end{center}

\section{Code examples}\label{sec:code_examples}
This section provides quantum programs for \emph{Bell state} preparation written in different \umbrellatermpl{}. These examples show the different approaches and syntax adopted by the chosen \umbrellatermpl{}. Hence, they provide insights about how convenient it is to program quantum algorithms.  

\begin{lstlisting}[keywords={Circ,bit,gate,output}, caption=Bell state preparation in QWIRE., basicstyle = \tiny\ttfamily]
bell: Circ(1, bit $\otimes$ bit) = box () =>
    a <- gate init0 (); b <- gate init0 ();
    a' <- gate H a;
    (a'', b') <- gate CNOT (a',b)
    output (a'', b')
\end{lstlisting}

\begin{lstlisting}[keywords={DEFCIRCUIT}, morecomment={[l]\#}, caption=Bell state preparation in Quil., basicstyle = \tiny\ttfamily]
DEFCIRCUIT BELL Qm Qn:
    H Qm
    CNOT Qm Qn
    MEASURE 0 [0] # Measurement results written to
    MEASURE 1 [1] # memory cells 0 and 1, respectively
\end{lstlisting}

\begin{lstlisting}[keywords={include, measure, qubit, bit}, caption=Bell state preparation in OpenQASM~3., basicstyle = \tiny\ttfamily]
OPENQASM 3;
include "stdgates.inc";

qubit[2] q;
bit[2] c;
h q[0];
cx q[0], q[1];
measure q -> c;
\end{lstlisting}

\begin{lstlisting}[language=python, caption=Bell state preparation in Qiskit., basicstyle = \tiny\ttfamily]
from qiskit import QuantumCircuit, transpile
from qiskit.providers.aer import QasmSimulator

qc = QuantumCircuit(2, 2)
qc.h(0)
qc.cx(0,1)
qc.measure([0,1], [0,1])

backend = QasmSimulator() # could be any other backend
qc_compiled = transpile(qc, backend)
job = backend.run(qc_compiled, shots=1024)
result = job.result()
\end{lstlisting}

\begin{lstlisting}[language=c++, caption=Bell state preparation in XACC., basicstyle = \tiny\ttfamily]
#include "xacc.hpp"
int main() {
  xacc::Initialize(argc, argv);
  auto accelerator = xacc::getAccelerator("qpp");
  auto buffer = xacc::qalloc(2);
  auto compiler = xacc::getCompiler("staq");
  auto ir = compiler->compile(R"(__qpu__ void bell(qbit q) {
H 0
CX 0 1
MEASURE 0 [0]
MEASURE 1 [1]
})", accelerator);
  accelerator->execute(buffer, ir->getComposites()[0]);
  buffer->print();
  xacc::Finalize();
}
\end{lstlisting}

\begin{lstlisting}[language=c++, caption=Bell state preparation in QCOR., basicstyle = \tiny\ttfamily]
__qpu__ void bell(qubit q, qubit r) {
  H(q);
  X::ctrl(q, r);
  Measure(q);
  Measure(r);
}
int main() {
  set_shots(1024);
  auto q = qalloc(2);
  bell(q[0], q[1]);
}
\end{lstlisting}

\begin{lstlisting}[language=c++, caption=Bell state preparation in OpenQL with C++ API (almost identical Python API exists as well)., basicstyle = \tiny\ttfamily]
#include <openql>

int main() {
    auto platf = ql::Platform("my_platform", "none");
    auto prog = ql::Program("bell", platf, 2);
    auto k = ql::Kernel("bell_kernel", platf, 2);
    k.prepz(0);
    k.prepz(0);
    k.hadamard(0);
    k.cnot(0, 1);
    k.measure(0);
    k.measure(1);
    prog.add_kernel(k);
    prog.compile();
}
\end{lstlisting}
\begin{lstlisting}[keywords={import,operation,return,bool, qubit},caption = Bell state preparation in Quingo., basicstyle = \tiny\ttfamily]
import config.json.*
import operations.*

operation bell(): bool[] {
    bool[2] result;
    using(q: qubit[2]) {
        init_all(q);
        H(q[0]);
        CNOT(q[0], q[1])
        result = meas_all(q);
    }
    return result;
}
\end{lstlisting}
\begin{lstlisting}[keywords={let,in},caption=Bell state preparation in Qunity., basicstyle = \tiny\ttfamily]
bell () := 
    let x $=_{\text{Bit}}$ (had 0) in $\Biggl($ctrl (x) $\begin{matrix} \\ _{\text{Bit}}\end{matrix}$$\left\lbrace\begin{array}{lll} 0 &\mapsto& (0, 0) \\ 1 &\mapsto& (1, 1)\end{array}\right\rbrace_{\text{Bit} \otimes  \text{Bit}}$ $\Biggr)$
\end{lstlisting}

\section{Overview of theoretical QPTs}\label{app:sec:qpts_without}%
\autoref{tab:qpts_without} lists the \umbrellatermpl{} that are not supported by a compilation toolchain. 
\begin{table}[H]
    \tiny
    \newcolumntype{P}[1]{>{\raggedright\arraybackslash}p{#1}}
    \begin{minipage}{\linewidth}%
    \centering
    \caption{Overview of \umbrellatermpl{} without compilation toolchain support.}
    \label{tab:qpts_without}
    \begin{tabular}{cP{2.9cm}P{1.6cm}P{2cm}P{1.9cm}P{1.5cm}}
    \toprule
        Year & Name & Type & Host Language & Paradigm & Execution Model\\
    \midrule
        1996 & Quantum Lambda Calculus~\cite{maymin_extending_1997} & Language & Lambda Calculus & Functional &  \\
        2000 & qGCL~\cite{sanders2000quantum} & Extension & pGCL & Imperative & QRAM \\
        2005 & QPAlg~\cite{jorrand2003, lalire_qpalg_2004} & Language & Extends (i.e., quantumize) Process Algebra & Process Algebra & QRAM \\
        2013 & Chisel-Q~\cite{liu_chisel-q_2013} & Framework & Scala & Functional & -\footnote{ends on QASM\label{fn:gen_2}} \\
        2013 & Quipper~\cite{green_quipper_2013} & Library & Haskell & Functional & Restricted \\
        2015 & Proto-Quipper~\cite{ross_algebraic_2017} & Language & Haskell & Functional & Restricted \\
        2016 & FJQuantum~\cite{feitosa_fjquantum_2016} & Language & Feather-weight Java & Imperative & QRAM \\
        2017 & QPCF~\cite{paolini_qpcf_2017} & Language & PCF & Functional & QRAM \\
        2018 & Q|SI>~\cite{liu_qsirangle_2017} & Framework & While-language \& C\# & Imperative & Restricted \\
        2019 & IQu~\cite{paolini_quantum_2019} & Language & Idealized Algol & Imperative\footnote{with functional elements\label{fn:gen_3}} & QRAM \\
        2020 & EWire~\cite{rennela_ewire_2020} &  & Lambda Calculus & Functional &  \\
        2020 & Silq~\cite{bichsel_silq_2020} & Language &  & Imperative\footref{fn:gen_3} & QRAM \\
        2022 & Qunity~\cite{voichick_qunity_2022} & Language &  & Functional &  \\
    \bottomrule
    \end{tabular}
    \end{minipage}
\end{table}

\section{Analysis Blueprint Evaluation}

\begin{table}[t]
    \tiny
    \centering
    \caption{Sample evaluation of Qiskit~\cite{qiskit} following the \textit{analysis blueprint}.}
    \label{tab:qiskit_blueprint}
    \begin{tabular}{llr}
    \toprule
        Question &  Answer & Rating\\
    \midrule
        Is it implemented? & Yes & - \\
        What is the type? & Library & - \\
        What is the host language? & Python &  - \\ \midrule
        Is the host language compiled or interpreted? & Interpreted & - \\
        Does it have language bindings? & Yes & - \\
        For which languages? & Rust, C++ & 6 \\ \midrule
        Are there addressable qubit registers? & Yes & - \\
        Does it provide a hardware interface? & No & - \\
        How is data transferred to the \gls{QPU}? & Binary Executable & 7\\ \midrule
        Are there any additional tools? & Multiple, e.g., VF2++, SabreSwap, ALAP/ASAP Scheduling ...  & --- \\
        How well are they implemented? & Well implemented, partly \gls{HPC} & 9 \\ \midrule
        How does it perform on large problems? & Sufficient, but single node &  6\\ \midrule
        Are real \glspl{QPU} supported? & Yes, can submit programs to multiple \glspl{QPU} in parallel & - \\
        Are different kinds of \glspl{QPU} supported? & Yes & 6 \\ \midrule
        What is the quantum memory model? & Shared, per \gls{QPU} & - \\ 
        What is the classical memory model? & Shared &  4\\ \midrule
        Who controls resource allocation? & The system & -\\
        Which types of resources are discriminated? & Classical and local \glspl{QPU} & 3\\ \midrule
        Can it easily be integrated with existing code? & No, since no header file exists& 3\\
    \bottomrule
    \end{tabular}
\end{table}
